# Supplementary material for: The Physics of Mergers: Theoretical and Statistical Techniques Applied to Stellar Mergers in Dense Star Clusters
Source: arXiv:1108.0662 source file (2011-08-02)
Supplement: Supplementary file 5 [file Dedication.tex]

\thispagestyle{empty}

%\begin{center}
%\vspace*{1.25in}

%{\it \LARGE\textsf{\`A ma m\`ere Carmelle et mon p\`ere Pierre, que nous
%n'oublirons jamais}}

%\hspace{1.85in}{\it \LARGE\textsf{\`A la m\'emoire de mon p\`ere, Pierre}\\}

\hspace{1.85in}{\it \LARGE\textsf{To my parents}\\}

%\vspace{0.25in}
%{\it \`A ma ch\`ere m\`ere, Carmelle}

%\end{center}
